# Supplementary material for: Evidence of scale-free clusters of vegetation in tropical rainforests
Source: arXiv:2301.05917 source file (2024-02-26)
Supplement: Supplementary file 1 [file 1-SuppInf_Clusters.pdf]

# Supplementary information: Evidence of scale-free clusters of vegetation in tropical rainforests

Pablo Villegas,<sup>1,\*</sup> Tommaso Gili,<sup>2</sup> Guido Caldarelli,<sup>3,4,5,6,7</sup> and Andrea Gabrielli<sup>1,8</sup>

<sup>1</sup>*‘Enrico Fermi’ Research Center (CREF), Via Panisperna 89A, 00184 - Rome, Italy*

<sup>2</sup>*Networks Unit, IMT Scuola Alti Studi Lucca, Piazza San Francesco 15, 55100- Lucca, Italy.*

<sup>3</sup>*DMSN, Ca’ Foscari University of Venice, Via Torino 155, 30172 - Venice, Italy*

<sup>4</sup>*European Centre for Living Technology (ECLT), Dorsoduro 3911, 30123 - Venice, Italy*

<sup>5</sup>*Institute for Complex Systems (ISC), CNR, UoS Sapienza, Piazzale Aldo Moro 2, 00185 - Rome, Italy*

<sup>6</sup>*London Institute for Mathematical Sciences (LIMS), W1K2XF London, United Kingdom*

<sup>7</sup>*Fondazione per il Futuro delle Città (FFC), Via Boccaccio 50, 50133 - Firenze Italy*

<sup>8</sup>*Dipartimento di Ingegneria, Università degli Studi ‘Roma Tre’, Via Vito Volterra 62, 00146 - Rome, Italy*

## CONTENTS

|                                                               |   |
|---------------------------------------------------------------|---|
| I. Distribution of cluster sizes for different species in BCI | 2 |
| A. Most abundant species                                      | 2 |
| B. Expanding species                                          | 3 |
| C. Contracting species                                        | 5 |

---

\* Corresponding author: [pablo.villegas@cref.it](mailto:pablo.villegas@cref.it)

# I. DISTRIBUTION OF CLUSTER SIZES FOR DIFFERENT SPECIES IN BCI

## A. Most abundant species

We present further analyses based on some of the most abundant species in Barro Colorado Island. As shown in Figure 1 and 2 the reported results for *H. prunifolius* are robust for some of the most abundant species in BCI. In particular, both *Tetragastris panamensis* and *Trichilia tuberculata* are part of the group of the 10 most abundant species, showing an intermediate state with scale-free clusters of vegetation.

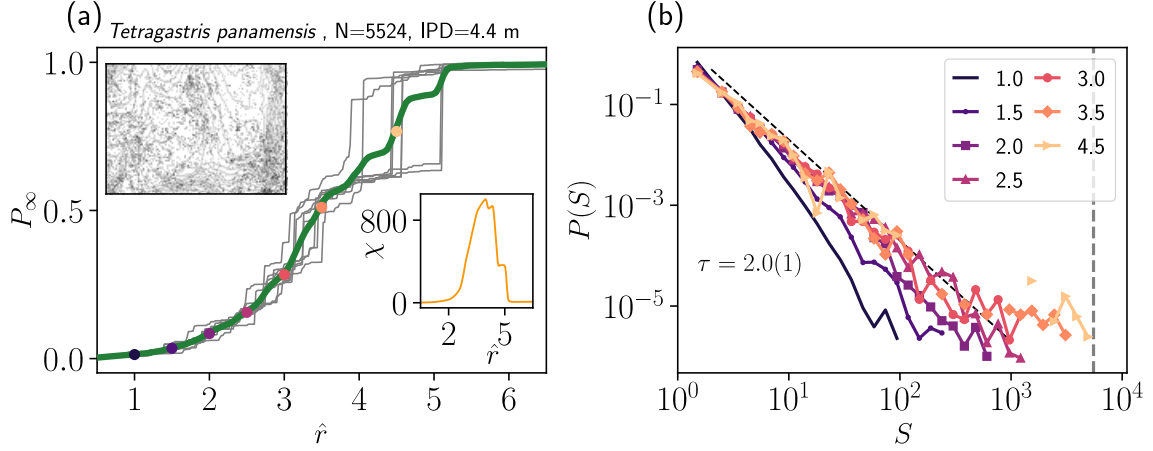

FIG. 1. *Tetragastris panamensis*. (a)  $P_\infty$  as a function of the distance parameter  $\hat{r}$ . Green line shows the average phase transition over the eight censuses from 1985 to 2005, while grey lines stand for individual censuses. Colored dots stand for the position where cluster size distributions are shown. Lower inset: Averaged system susceptibility. A non-trivial extended region with high susceptibility, ranging into  $\hat{r} \in (2, 4)$ , can be appreciated. Upper inset: Spatial distribution for Census 8. (b) Cluster size distribution averaged over all censuses for different values of  $\hat{r}$  (see legend). There exists an intermediate (critical) region with variable exponents. Dashed lines are guides to the eye representing  $\tau = 2.0$ .

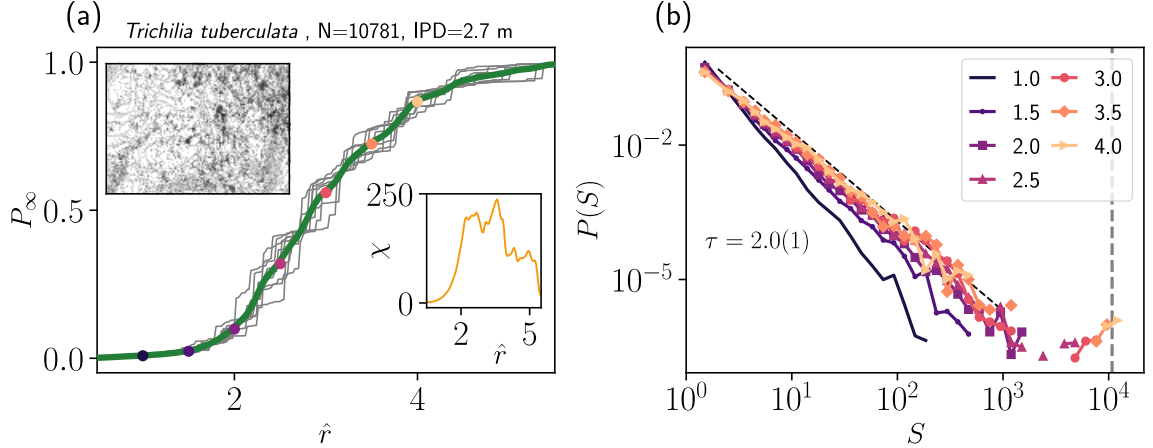

FIG. 2. *Trichilia tuberculata*. (a)  $P_\infty$  as a function of the distance parameter  $\hat{r}$ . Green line shows the average phase transition over the eight censuses from 1985 to 2005, while grey lines stand for individual censuses. Colored dots stand for the position where cluster size distributions are shown. Lower inset: Averaged system susceptibility. A non-trivial extended region with high susceptibility, ranging into  $\hat{r} \in (2, 5)$ , can be appreciated. Upper inset: Spatial distribution for Census 8. (b) Cluster size distribution averaged over all censuses for different values of  $\hat{r}$  (see legend). There exists an intermediate (critical) region with variable exponents. Dashed lines are guides to the eye representing  $\tau = 2.0$ .

### B. Expanding species

We present here results for two of the most notable cases of expanding species in BCI. In particular we select *Eugenia galalonensis* (it has risen from  $N = 964$  stems in Census 1 to  $N = 2400$  stems in Census 8) and *Calophyllum longifolium* (it has risen from  $N = 647$  stems in Census 1 to  $N = 2237$  stems in Census 8).

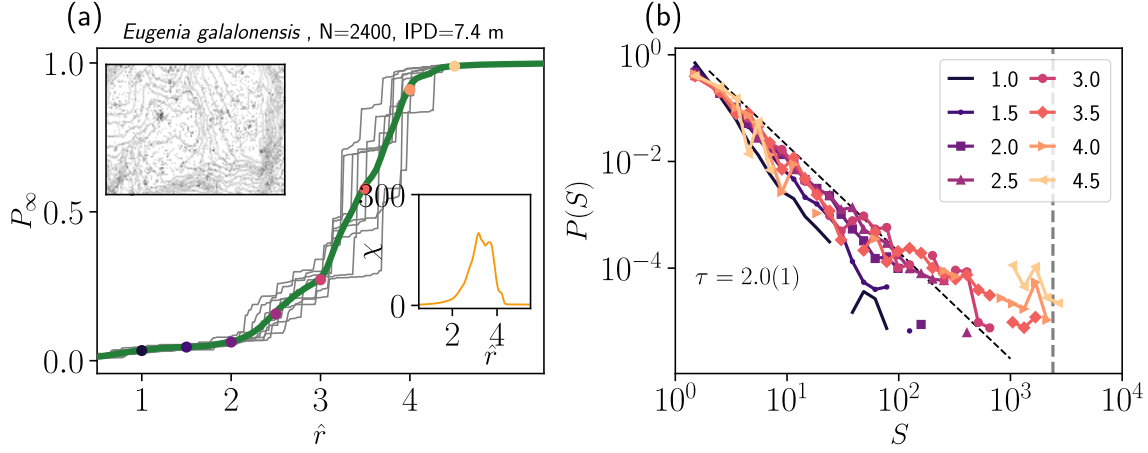

FIG. 3. *Eugenia galalonensis*. (a)  $P_\infty$  as a function of the distance parameter  $\hat{r}$ . Green line shows the average phase transition over the eight censuses from 1985 to 2005, while grey lines stand for individual censuses. Colored dots stand for the position where cluster size distributions are shown. Lower inset: Averaged system susceptibility. A non-trivial extended region with high susceptibility, ranging into  $\hat{r} \in (2, 5)$ , can be appreciated. Upper inset: Spatial distribution for Census 8. (b) Cluster size distribution averaged over all censuses for different values of  $\hat{r}$  (see legend). There exists an intermediate (critical) region with variable exponents. Dashed lines are guides to the eye representing  $\tau = 2.0$ .

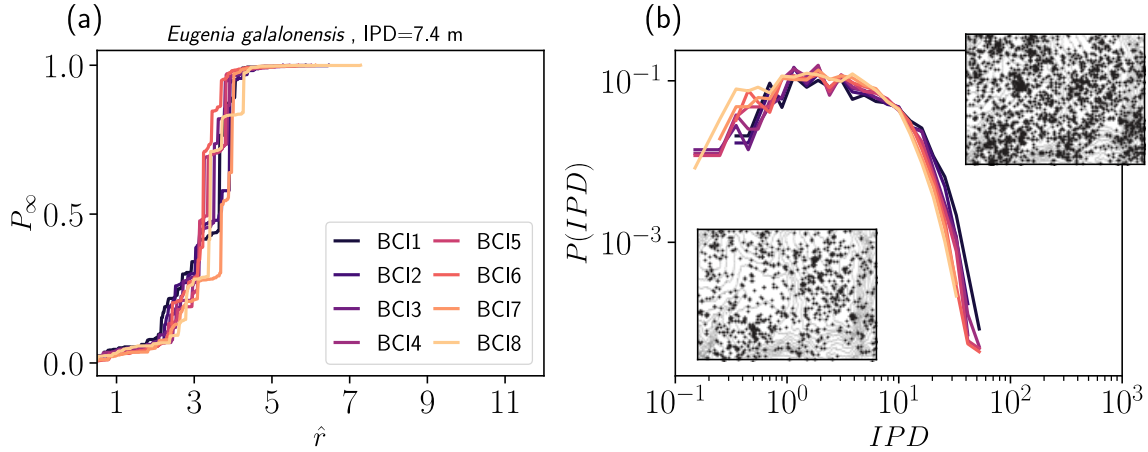

FIG. 4. *Eugenia galalonensis*. (a)  $P_\infty$  as a function of the distance parameter  $\hat{r}$  for the eight censuses from 1985 to 2005 (see legend). (b) Mean-nearest neighbor distance probability distribution for the different censuses. Insets: Species spatial distribution for Census 1 (lower inset) and Census 8 (upper inset), respectively.

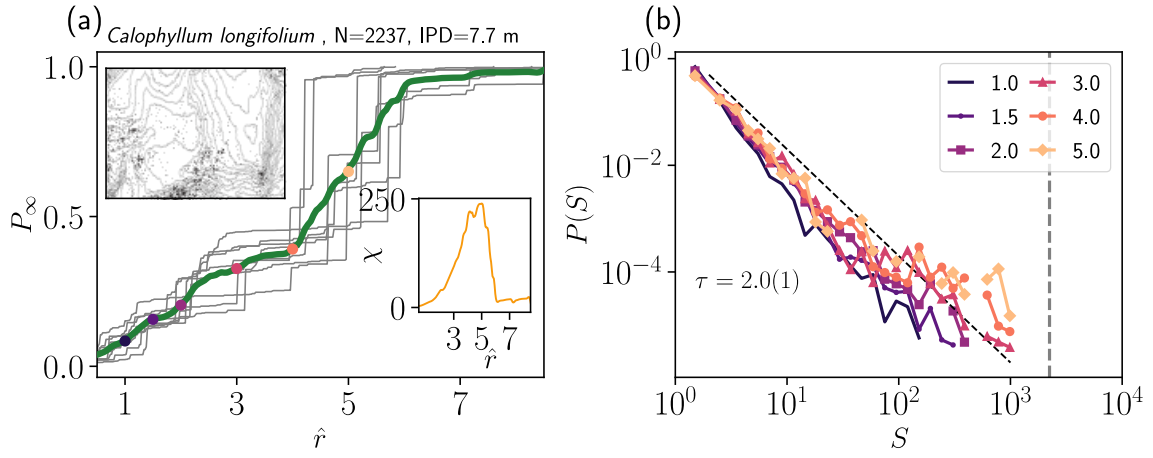

FIG. 5. *Calophyllum longifolium*. (a)  $P_\infty$  as a function of the distance parameter  $\hat{r}$ . Green line shows the average phase transition over the eight censuses from 1985 to 2005, while grey lines stand for individual censuses. Colored dots stand for the position where cluster size distributions are shown. Lower inset: Averaged system susceptibility. A non-trivial extended region with high susceptibility, ranging into  $\hat{r} \in (2, 5)$ , can be appreciated. Upper inset: Spatial distribution for Census 8. (b) Cluster size distribution averaged over all censuses for different values of  $\hat{r}$  (see legend). There exists an intermediate (critical) region with variable exponents. Dashed lines are guides to the eye representing  $\tau = 2.0$ .

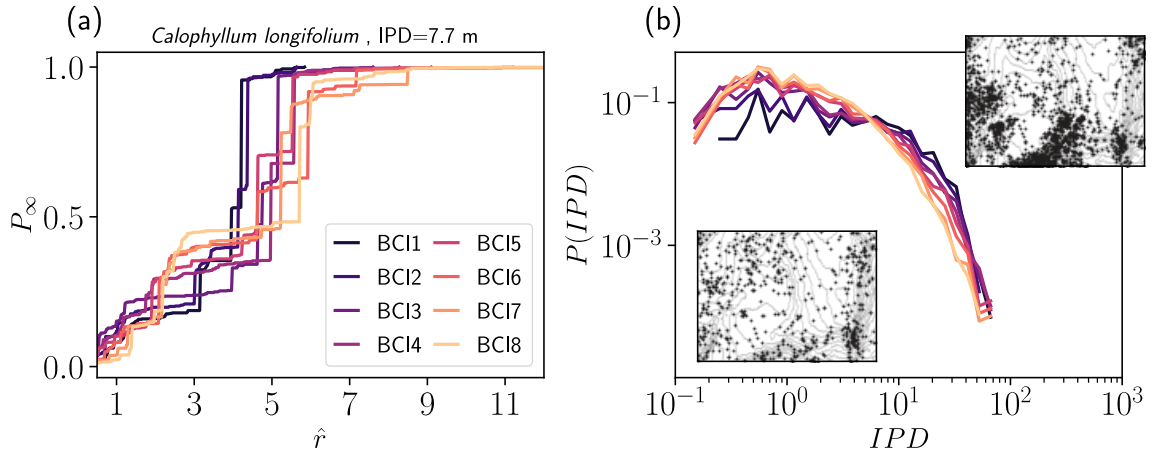

FIG. 6. *Eugenia galanensis*. (a)  $P_\infty$  as a function of the distance parameter  $\hat{r}$  for the eight censuses from 1985 to 2005 (see legend). (b) Mean-nearest neighbor distance probability distribution for the different censuses. Insets: Species spatial distribution for Census 1 (lower inset) and Census 8 (upper inset), respectively.

### C. Contracting species

We present here results for two of the most notable cases of contracting species in BCI. In particular we select *Piper cordulatum* (it has risen from  $N = 3142$  stems in Census 1 to  $N = 98$  stems in Census 8) and *Psychotria horizontalis* (it has risen from  $N = 6159$  stems in Census 1 to  $N = 1856$  stems in Census 8).

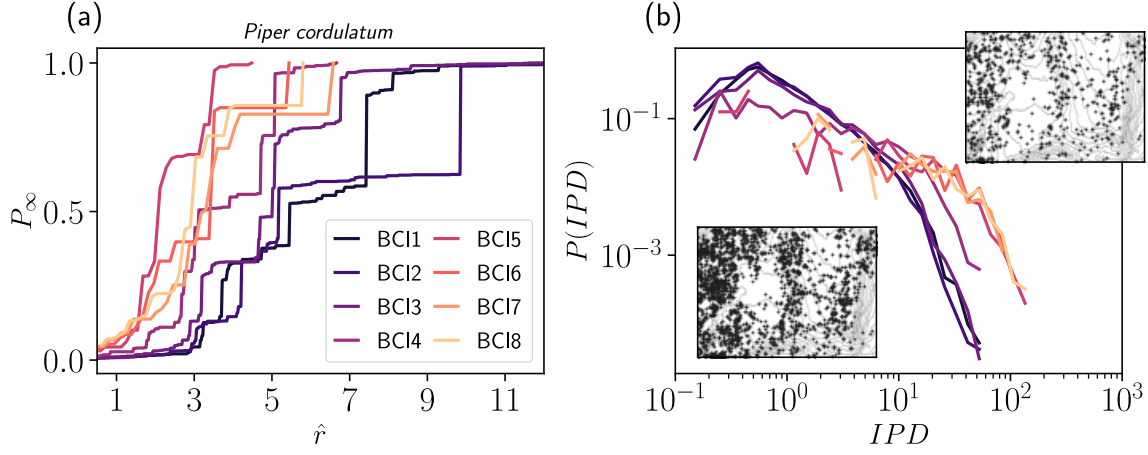

FIG. 7. *Piper cordulatum*. (a)  $P_\infty$  as a function of the distance parameter  $\hat{r}$  for the eight censuses from 1985 to 2005 (see legend). (b) Mean-nearest neighbor distance probability distribution for the different censuses. Insets: Species spatial distribution for Census 3 (lower inset) and Census 4 (upper inset), respectively.

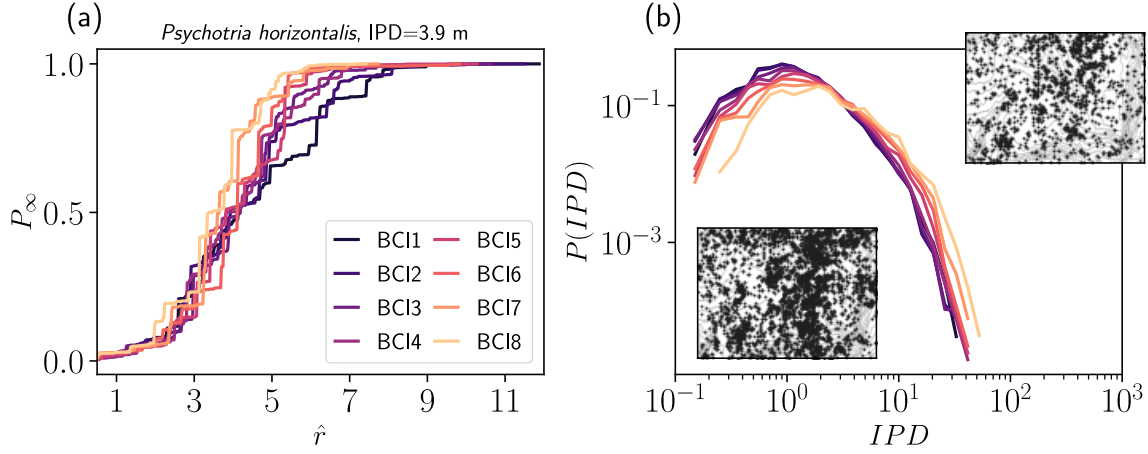

FIG. 8. *Psychotria horizontalis*. (a)  $P_\infty$  as a function of the distance parameter  $\hat{r}$  for the eight censuses from 1985 to 2005 (see legend). (b) Mean-nearest neighbor distance probability distribution for the different censuses. Insets: Species spatial distribution for Census 3 (lower inset) and Census 4 (upper inset), respectively.
